# Supplementary material for: Nondestructive characterization of laser-cooled atoms using machine learning
Source: arXiv:2509.26479 source file (2025-09-30)
Supplement: Supplementary file 1 [file SM.pdf]

# Nondestructive characterization of laser-cooled atoms using machine learning

G. De Sousa 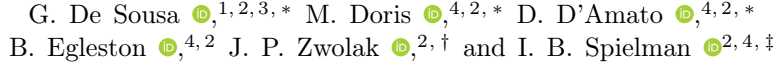<sup>1,2,3,\*</sup> M. Doris 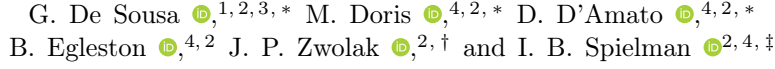<sup>4,2,\*</sup> D. D'Amato 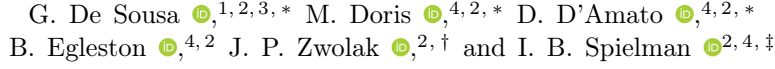<sup>4,2,\*</sup>  
B. Egleston 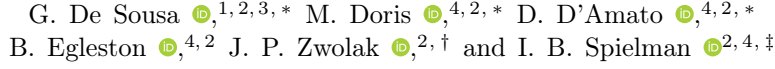<sup>4,2</sup> J. P. Zwolak 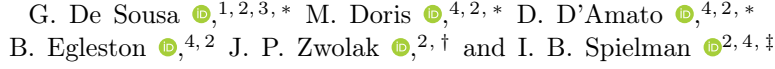<sup>2,†</sup> and I. B. Spielman 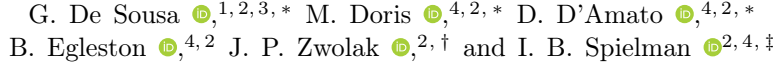<sup>2,4,‡</sup>

<sup>1</sup>*Department of Physics, University of Maryland, College Park, MD 20742, USA*

<sup>2</sup>*National Institute of Standards and Technology, Gaithersburg, Maryland, 20899, USA*

<sup>3</sup>*Instituto de Física de São Carlos, Universidade de São Paulo, 13560-970, São Carlos, SP, Brasil*

<sup>4</sup>*Joint Quantum Institute, National Institute of Standards and Technology  
and University of Maryland, Gaithersburg, Maryland 20899, USA*

(Dated: September 30, 2025)

## I. IMAGING DETAILS

The raw fluorescence images are recorded by briefly collecting light emitted by the laser-cooled atoms onto our  $\mathbf{e}_x$  and  $\mathbf{e}_z$  cameras; these images inevitably include a non-negligible background of scattered laser light and ambient room light. To mitigate this, we subtract a second reference frame taken under otherwise identical conditions but without atoms.

Each TOF absorption image of 2D column density  $\rho_{\mathbf{i}}$  is assembled from three image frames in raw ADUs (analog to digital units) from the  $\mathbf{e}_y$  camera: an “atoms” frame  $N_{\mathbf{i}}^{\text{at}}$ , a probe-only frame  $N_{\mathbf{i}}^{\text{pr}}$ , and a background frame  $N_{\mathbf{i}}^{\text{bg}}$ . Here, we label pixels by their vector coordinate  $\mathbf{i} = (i, j)$ . In the atoms frame, the TOF-expanded cloud is illuminated by the probe laser for 10  $\mu\text{s}$ . The probe frame is a replica of the atoms frame, but with no atoms present. Finally, we record the background frame with the probe laser turned off, but all other conditions kept the same.

Together, these frames yield the column density

$$\rho_{\mathbf{i}} = -\frac{1}{\sigma_0} \left[ \log \left( \frac{N_{\mathbf{i}}^{\text{at}} - N_{\mathbf{i}}^{\text{bg}}}{N_{\mathbf{i}}^{\text{pr}} - N_{\mathbf{i}}^{\text{bg}}} \right) - \frac{N_{\mathbf{i}}^{\text{at}} - N_{\mathbf{i}}^{\text{pr}}}{N_{\text{sat}}} \right], \quad (\text{SM-1})$$

where  $\sigma_0 = 3\lambda^2/(2\pi)$  is the resonant scattering cross-sections for the imaging transition at wavelength  $\lambda = 766.7$  nm and  $N_{\text{sat}} = 200$  (obtained as in Refs. 1 and 2) is the number of ADUs corresponding to the saturation intensity  $I_{\text{sat}} = 1.75$  mW/cm<sup>2</sup>.

## II. NUMBER AND TEMPERATURE LABELING

The number and temperature labels are determined from joint fits to all  $M$  absorption images within a given set (labeled by  $k = 1, \dots, M$ ) of column density  $\rho_{\mathbf{i}}^{(k)}$  to a TOF-dependent Gaussian profile whose width increases in time  $t_{\text{TOF}}^{(k)}$ .

We model the initial  $t_{\text{TOF}} = 0$  density distribution with a Gaussian profile, and further assume that the velocity is thermally distributed (i.e., also Gaussian). The TOF-expansion along the  $\mathbf{e}_x$  and  $\mathbf{e}_z$  directions (observed by our “ $\mathbf{e}_y$ ” TOF camera) is observed to be anisotropic, necessitating different “temperature” parameters  $T_x$  and  $T_z$ . All together, this leads to a model distribution that is Gaussian at all times with widths

$$w_j^2(t_{\text{TOF}}) = w_j^2(0) + \frac{k_B T_j}{m} t_{\text{TOF}}^2, \quad \text{with} \quad j \in \{x, z\}, \quad (\text{SM-2})$$

where  $w_j(0)$  denotes the initial size of the cloud. In what follows we generalize the notation  $t_{\text{TOF}}^{(k)}$  introduced for TOF-times to compactly label quantities associated with our specific observation times, i.e.,  $w_j \left( t_{\text{TOF}}^{(k)} \right) \rightarrow w_j^{(k)}$ . We use (0) to denote (unobserved) quantities at  $t_{\text{TOF}} = 0$ .

---

\* These authors contributed equally to this work.

† jpzwolak@nist.gov

‡ ian.spielman@nist.gov

These definitions lead to the fit function for TOF density distributions imaged on our CCD camera

$$n_{\mathbf{i}}^{(k)} = N \left[ 2\pi \prod_{j \in x,z} w_j^{(k)} \right]^{-1} \exp \left[ -\frac{1}{2} \sum_{j \in x,z} \left( \frac{r_j - r_{0,j}^{(k)}}{w_j^{(k)}} \right)^2 \right]. \quad (\text{SM-3})$$

where pixels sample positions  $(x, z) \equiv \mathbf{r} = \Delta x \mathbf{i}$ ;  $\Delta x$  is the magnified and down-sampled pixel size; and  $r_{0,j}^{(k)}$  is the spatial center of the distribution. The spatial center

$$\mathbf{r}_0^{(k)} = \mathbf{r}_0 + \mathbf{v} t_{\text{TOF}}^{(k)} + \delta_{k,1} \mathbf{r}_{\text{step}} \quad (\text{SM-4})$$

was specified by fit parameters: an initial position  $\mathbf{r}_0$ , an initial velocity  $\mathbf{v}$ , and a small offset  $\mathbf{r}_{\text{step}}$  ( $\delta_{k,1}$  is the Kronecker- $\delta$  function). We introduced  $\mathbf{r}_{\text{step}}$  to account for a systematic shift in the center position of the cloud in the 1 ms images; this shift was found to be only along  $\mathbf{e}_z$ .

We then minimize the objective function

$$E = \sum_k \sum_{\mathbf{i}} \left[ \frac{\rho_{\mathbf{i}}^{(k)} - n_{\mathbf{i}}^{(k)}}{\Sigma_{\mathbf{i}}^{(k)}} \right]^2, \quad (\text{SM-5})$$

to determine the fit parameters; each contribution to  $E$  is weighted by pixel-by-pixel uncertainties  $\Sigma_{\mathbf{i}}^{(k)}$  derived from photon shot noise in the individual images used in absorption imaging. We minimized with respect to the parameters  $(N, T_x, T_y, w_x^{(0)}, w_z^{(0)}, r_{0,z}, v_z, r_{\text{step},z})$  and found that the remaining parameters  $(r_{0,x}, v_x, r_{\text{step},x})$  were constant across the dataset, within the uncertainties. This lead to our final labels  $N$  and  $T = (T_x + T_z)/2$ .

---

[1] G. Reinaudi, T. Lahaye, Z. Wang, and D. Guéry-Odelin, Opt. Lett. **32**, 3143 (2007).

[2] E. M. Seroka, A. V. Curiel, D. Trypogeorgos, N. Lundblad, and I. B. Spielman, Opt. Express **27**, 36611 (2019).

TABLE SM-I. Architectures of all models used in this work. All Dense layers are assumed to include bias, and the number inside the parentheses of the Conv2D layer indicates the size of the kernel. The notation LeakyReLU\* indicates BatchNorm2D  $\rightarrow$  LeakyReLU  $\rightarrow$  Dropout(0.2), and is used during training.

| CON, # parameters = 4 |                   |                             |            | LIN, # parameters = 12      |                             |            |                             | MM, # parameters = 24580    |                             |            |                              | MLP, # parameters = 7840036  |                              |            |                                         | CNN, # parameters = 1397156             |                                         |                                         |                                         |
|-----------------------|-------------------|-----------------------------|------------|-----------------------------|-----------------------------|------------|-----------------------------|-----------------------------|-----------------------------|------------|------------------------------|------------------------------|------------------------------|------------|-----------------------------------------|-----------------------------------------|-----------------------------------------|-----------------------------------------|-----------------------------------------|
| Layer type            | Size              | Size                        | Layer type | Size                        | Size                        | Layer type | Size                        | Size                        | Size                        | Layer type | Size                         | Size                         | Size                         | Layer type | Size                                    | Size                                    | Size                                    | Size                                    | Size                                    |
| Input                 | -                 | -                           | Input      | (64, 48)                    | (64, 48)                    | Input      | (64, 48)                    | (64, 48)                    | (64, 48)                    | Input      | (64, 48)                     | (64, 48)                     | (64, 48)                     | Input      | (64, 48)                                | (64, 48)                                | (64, 48)                                | (64, 48)                                | (64, 48)                                |
| Linear                | 0 $\rightarrow$ 4 | (64, 48) $\rightarrow$ 3072 | Flatten    | (64, 48) $\rightarrow$ 3072 | (64, 48) $\rightarrow$ 3072 | Flatten    | (64, 48) $\rightarrow$ 3072 | (64, 48) $\rightarrow$ 3072 | (64, 48) $\rightarrow$ 3072 | Flatten    | (64, 48) $\rightarrow$ 3072  | (64, 48) $\rightarrow$ 3072  | (64, 48) $\rightarrow$ 3072  | Conv2D(9)  | (1, 64, 48) $\rightarrow$ (8, 64, 48)   | (1, 64, 48) $\rightarrow$ (8, 64, 48)   | (1, 64, 48) $\rightarrow$ (8, 64, 48)   | (1, 64, 48) $\rightarrow$ (8, 64, 48)   | (1, 64, 48) $\rightarrow$ (8, 64, 48)   |
| Output                | 4                 | 3072 $\rightarrow$ 1        | Sum        | (64, 48) $\rightarrow$ 3072 | (64, 48) $\rightarrow$ 3072 | Fuse       | (64, 48) $\rightarrow$ 3072 | (64, 48) $\rightarrow$ 3072 | (64, 48) $\rightarrow$ 3072 | Linear     | (64, 48) $\rightarrow$ 3072  | (64, 48) $\rightarrow$ 3072  | (64, 48) $\rightarrow$ 3072  | LeakyReLU* | (8, 64, 48) $\rightarrow$ (8, 32, 24)   | (8, 64, 48) $\rightarrow$ (8, 32, 24)   | (8, 64, 48) $\rightarrow$ (8, 32, 24)   | (8, 64, 48) $\rightarrow$ (8, 32, 24)   | (8, 64, 48) $\rightarrow$ (8, 32, 24)   |
|                       |                   | (1, 1) $\rightarrow$ 2      | Fuse       | (1, 1) $\rightarrow$ 2      | (1, 1) $\rightarrow$ 2      | Linear     | (1, 1) $\rightarrow$ 2      | (1, 1) $\rightarrow$ 2      | (1, 1) $\rightarrow$ 2      | Linear     | (1, 1) $\rightarrow$ 2       | (1, 1) $\rightarrow$ 2       | (1, 1) $\rightarrow$ 2       | Conv2D(9)  | (8, 32, 24) $\rightarrow$ (16, 32, 24)  | (8, 32, 24) $\rightarrow$ (16, 32, 24)  | (8, 32, 24) $\rightarrow$ (16, 32, 24)  | (8, 32, 24) $\rightarrow$ (16, 32, 24)  | (8, 32, 24) $\rightarrow$ (16, 32, 24)  |
|                       |                   | 2 $\rightarrow$ 4           | Linear     | 2 $\rightarrow$ 4           | 2 $\rightarrow$ 4           | Output     | 2 $\rightarrow$ 4           | 2 $\rightarrow$ 4           | 2 $\rightarrow$ 4           | Linear     | 2 $\rightarrow$ 4            | 2 $\rightarrow$ 4            | 2 $\rightarrow$ 4            | LeakyReLU* | (16, 32, 24) $\rightarrow$ (16, 32, 24) | (16, 32, 24) $\rightarrow$ (16, 32, 24) | (16, 32, 24) $\rightarrow$ (16, 32, 24) | (16, 32, 24) $\rightarrow$ (16, 32, 24) | (16, 32, 24) $\rightarrow$ (16, 32, 24) |
|                       |                   | 4                           | Output     | 4                           | 4                           |            | 4                           | 4                           | 4                           | Linear     | 4                            | 4                            | 4                            | AvgPool2d  | (16, 32, 24) $\rightarrow$ (16, 16, 12) | (16, 32, 24) $\rightarrow$ (16, 16, 12) | (16, 32, 24) $\rightarrow$ (16, 16, 12) | (16, 32, 24) $\rightarrow$ (16, 16, 12) | (16, 32, 24) $\rightarrow$ (16, 16, 12) |
|                       |                   |                             |            |                             |                             |            |                             |                             |                             | LeakyReLU  |                              |                              |                              | Conv2D(9)  | (16, 16, 12) $\rightarrow$ (32, 16, 12) | (16, 16, 12) $\rightarrow$ (32, 16, 12) | (16, 16, 12) $\rightarrow$ (32, 16, 12) | (16, 16, 12) $\rightarrow$ (32, 16, 12) | (16, 16, 12) $\rightarrow$ (32, 16, 12) |
|                       |                   |                             |            |                             |                             |            |                             |                             |                             | Fuse       | (256, 256) $\rightarrow$ 512 | (256, 256) $\rightarrow$ 512 | (256, 256) $\rightarrow$ 512 | LeakyReLU* | (32, 16, 12) $\rightarrow$ (32, 8, 6)   | (32, 16, 12) $\rightarrow$ (32, 8, 6)   | (32, 16, 12) $\rightarrow$ (32, 8, 6)   | (32, 16, 12) $\rightarrow$ (32, 8, 6)   | (32, 16, 12) $\rightarrow$ (32, 8, 6)   |
|                       |                   |                             |            |                             |                             |            |                             |                             |                             | Linear     | 512 $\rightarrow$ 256        | 512 $\rightarrow$ 256        | 512 $\rightarrow$ 256        | AvgPool2d  | (32, 8, 6) $\rightarrow$ (64, 8, 6)     | (32, 8, 6) $\rightarrow$ (64, 8, 6)     | (32, 8, 6) $\rightarrow$ (64, 8, 6)     | (32, 8, 6) $\rightarrow$ (64, 8, 6)     | (32, 8, 6) $\rightarrow$ (64, 8, 6)     |
|                       |                   |                             |            |                             |                             |            |                             |                             |                             | LeakyReLU  | 256 $\rightarrow$ 256        | 256 $\rightarrow$ 256        | 256 $\rightarrow$ 256        | Conv2D(9)  | (64, 8, 6) $\rightarrow$ (64, 4, 3)     | (64, 8, 6) $\rightarrow$ (64, 4, 3)     | (64, 8, 6) $\rightarrow$ (64, 4, 3)     | (64, 8, 6) $\rightarrow$ (64, 4, 3)     | (64, 8, 6) $\rightarrow$ (64, 4, 3)     |
|                       |                   |                             |            |                             |                             |            |                             |                             |                             | Linear     | 256 $\rightarrow$ 128        | 256 $\rightarrow$ 128        | 256 $\rightarrow$ 128        | AvgPool2d  | (64, 4, 3) $\rightarrow$ 768            | (64, 4, 3) $\rightarrow$ 768            | (64, 4, 3) $\rightarrow$ 768            | (64, 4, 3) $\rightarrow$ 768            | (64, 4, 3) $\rightarrow$ 768            |
|                       |                   |                             |            |                             |                             |            |                             |                             |                             | LeakyReLU  | 128 $\rightarrow$ 32         | 128 $\rightarrow$ 32         | 128 $\rightarrow$ 32         | Flatten    | (768, 768) $\rightarrow$ 1536           | (768, 768) $\rightarrow$ 1536           | (768, 768) $\rightarrow$ 1536           | (768, 768) $\rightarrow$ 1536           | (768, 768) $\rightarrow$ 1536           |
|                       |                   |                             |            |                             |                             |            |                             |                             |                             | Linear     | 32 $\rightarrow$ 4           | 32 $\rightarrow$ 4           | 32 $\rightarrow$ 4           | Fuse       | 1536 $\rightarrow$ 512                  | 1536 $\rightarrow$ 512                  | 1536 $\rightarrow$ 512                  | 1536 $\rightarrow$ 512                  | 1536 $\rightarrow$ 512                  |
|                       |                   |                             |            |                             |                             |            |                             |                             |                             | LeakyReLU  | 4                            | 4                            | 4                            | Linear     | 512 $\rightarrow$ 256                   | 512 $\rightarrow$ 256                   | 512 $\rightarrow$ 256                   | 512 $\rightarrow$ 256                   | 512 $\rightarrow$ 256                   |
|                       |                   |                             |            |                             |                             |            |                             |                             |                             | Linear     | 256 $\rightarrow$ 128        | 256 $\rightarrow$ 128        | 256 $\rightarrow$ 128        | LeakyReLU  | 256 $\rightarrow$ 128                   | 256 $\rightarrow$ 128                   | 256 $\rightarrow$ 128                   | 256 $\rightarrow$ 128                   | 256 $\rightarrow$ 128                   |
|                       |                   |                             |            |                             |                             |            |                             |                             |                             | Output     |                              |                              |                              | LeakyReLU  | 128 $\rightarrow$ 64                    | 128 $\rightarrow$ 64                    | 128 $\rightarrow$ 64                    | 128 $\rightarrow$ 64                    | 128 $\rightarrow$ 64                    |
|                       |                   |                             |            |                             |                             |            |                             |                             |                             |            |                              |                              |                              | Linear     | 64 $\rightarrow$ 4                      | 64 $\rightarrow$ 4                      | 64 $\rightarrow$ 4                      | 64 $\rightarrow$ 4                      | 64 $\rightarrow$ 4                      |
|                       |                   |                             |            |                             |                             |            |                             |                             |                             |            |                              |                              |                              | Output     | 4                                       | 4                                       | 4                                       | 4                                       | 4                                       |

TABLE SM-II. Complete results for all models, including every training and testing augmentation. Each column contains a model trained with a different augmentation. For a given metric (FVU,  $\Delta T$ ,  $\Delta N$ ,  $\mathcal{F}_T$ ,  $\mathcal{F}_N$ ), each row shows the score of a trained model when tested with a given augmentation (U, T, R, RT). The numbers in parentheses show the most significant digit of the standard deviation.

|                              |          | In-distribution test set |           |           |           |                       |           |          |           |                       |                     |          |          |
|------------------------------|----------|--------------------------|-----------|-----------|-----------|-----------------------|-----------|----------|-----------|-----------------------|---------------------|----------|----------|
|                              |          | CON                      |           |           | LIN       |                       |           | MM       |           |                       | MLP                 |          |          |
| Testing                      | Training | CON                      |           |           | LIN       |                       |           | MM       |           |                       | MLP                 |          |          |
|                              |          | U                        | R         | T         | U         | R                     | T         | U        | R         | T                     | U                   | R        | T        |
| FVU                          | U        | 0.440(2)                 | 0.4394(5) | 0.4347(4) | 0.4364(7) | 0.868(1)              | 0.787(1)  | 0.493(1) | 0.448(2)  | 0.9703(2)             | 0.9704(4)           | 0.951(2) | 0.920(6) |
|                              | R        | 0.443(2)                 | 0.4437(5) | 0.4354(4) | 0.4375(7) | -3.2(2)               | 0.780(1)  | 0.439(2) | 0.453(1)  | -1.6(5)               | 0.9703(2)           | 0.47(6)  | 0.925(4) |
|                              | T        | 0.29(2)                  | 0.25(2)   | 0.435(1)  | 0.4355(9) | -3.0(2) $\times 10^2$ | -69(3)    | 0.513(2) | 0.474(4)  | -8(6) $\times 10^1$   | -6(4) $\times 10^1$ | 0.948(2) | 0.921(4) |
|                              | RT       | 0.30(2)                  | 0.29(1)   | 0.436(1)  | 0.437(1)  | -3.3(2) $\times 10^2$ | -66(4)    | 0.39(2)  | 0.478(3)  | -1.2(9) $\times 10^2$ | -5(3) $\times 10^1$ | 0.41(6)  | 0.922(4) |
| $\Delta T$ [mK]              | U        | 11.005(5)                | 10.99(1)  | 11.196(5) | 11.188(8) | 7.05(2)               | 8.32(2)   | 10.96(2) | 10.92(2)  | 2.70(8)               | 3.20(6)             | 4.27(5)  | 4.66(6)  |
|                              | R        | 10.968(6)                | 10.95(1)  | 11.192(5) | 11.181(8) | 8.75(6)               | 8.45(2)   | 11.00(2) | 10.96(1)  | 6.5(2)                | 3.22(7)             | 5.56(7)  | 4.73(5)  |
|                              | T        | 11.011(8)                | 10.75(1)  | 11.174(5) | 11.150(7) | 29.5(6)               | 16.2(2)   | 10.73(1) | 10.757(8) | 18(5)                 | 14(3)               | 4.46(4)  | 4.98(5)  |
|                              | RT       | 10.76(1)                 | 10.71(1)  | 11.168(6) | 11.144(7) | 30.7(5)               | 15.9(2)   | 10.71(2) | 10.76(1)  | 21(7)                 | 14(3)               | 5.77(7)  | 5.01(6)  |
| $\Delta N$ [ $\times 10^6$ ] | U        | 24.31(5)                 | 24.44(4)  | 23.75(2)  | 23.77(2)  | 11.87(7)              | 16.81(8)  | 22.17(2) | 23.09(3)  | 3.67(6)               | 3.8(1)              | 7.3(2)   | 10.3(5)  |
|                              | R        | 24.02(5)                 | 24.13(5)  | 23.57(2)  | 23.56(2)  | 62(1)                 | 16.5(1)   | 23.28(5) | 23.16(4)  | 22(1)                 | 3.75(7)             | 19.8(6)  | 10.0(4)  |
|                              | T        | 28.0(2)                  | 28.4(4)   | 23.94(5)  | 23.97(5)  | 274(9)                | 158(3)    | 23.11(9) | 24.1(1)   | 5(1) $\times 10^1$    | 43(3)               | 7.7(2)   | 10.4(4)  |
|                              | RT       | 27.7(2)                  | 28.1(2)   | 23.75(3)  | 23.82(5)  | 285(9)                | 158(3)    | 25.1(1)  | 23.76(7)  | 5(1) $\times 10^1$    | 42(3)               | 19.8(5)  | 10.4(4)  |
| $\mathcal{F}_T$              | U        | 0.7426(2)                | 0.7427(8) | 0.7516(2) | 0.7511(5) | 0.476(1)              | 0.559(1)  | 0.725(1) | 0.730(1)  | 0.56(6)               | 0.27(2)             | 0.40(6)  | 0.46(3)  |
|                              | R        | 0.7391(2)                | 0.7389(8) | 0.7512(2) | 0.7504(5) | 1.39(4)               | 0.5639(9) | 0.736(1) | 0.7330(8) | 1.4(1)                | 0.30(3)             | 0.65(3)  | 0.43(3)  |
|                              | T        | 0.765(5)                 | 0.774(4)  | 0.7505(4) | 0.7494(5) | 11.3(2)               | 5.40(8)   | 0.725(1) | 0.731(1)  | 7(2)                  | 6(2)                | 0.37(4)  | 0.39(3)  |
|                              | RT       | 0.758(3)                 | 0.761(4)  | 0.7498(4) | 0.7484(4) | 11.9(2)               | 5.4(1)    | 0.746(5) | 0.7302(9) | 7(3)                  | 5(1)                | 0.66(2)  | 0.39(3)  |
| $\mathcal{F}_N$              | U        | 1.068(6)                 | 1.048(4)  | 1.137(4)  | 1.122(5)  | 0.486(5)              | 0.573(3)  | 0.985(4) | 1.005(4)  | 0.169(7)              | 0.138(7)            | 0.26(2)  | 0.37(3)  |
|                              | R        | 1.078(6)                 | 1.058(4)  | 1.140(4)  | 1.125(5)  | 1.02(2)               | 0.563(5)  | 1.003(5) | 1.017(3)  | 0.59(2)               | 0.16(1)             | 0.60(3)  | 0.37(3)  |
|                              | T        | 1.102(7)                 | 1.086(6)  | 1.137(6)  | 1.124(5)  | 3.9(1)                | 2.20(4)   | 1.006(5) | 1.030(6)  | 0.8(2)                | 0.66(7)             | 0.27(1)  | 0.39(2)  |
|                              | RT       | 1.110(7)                 | 1.096(7)  | 1.139(5)  | 1.127(4)  | 3.9(1)                | 2.20(4)   | 1.009(5) | 1.036(4)  | 0.9(1)                | 0.66(6)             | 0.57(2)  | 0.39(2)  |
